# Supplementary material for: Lead-free CsSnCl$_{3}$ perovskite nanocrystals: Rapid synthesis, experimental characterization and DFT simulations
Source: arXiv:2111.00181 source file (2021-10-30)
Supplement: Supplementary file 1 [file appendix1.tex]

\section{Supplementary Material} \label{sec:appendix}
    Here the ESI will be included.
